# Supplementary material for: Spatial Reasoning via Deep Vision Models for Robotic Sequential Manipulation
Source: arXiv:2306.17053 source file (2023-08-01)
Supplement: Supplementary file 1 [file 7_Supplementary.tex]

\section{Supplementary Material}
% Define block styles
\tikzstyle{context_patches} = [rectangle, draw, fill=blue!20, inner sep=0.0mm,
    text width=10em, text height = 1.8cm, text centered, rounded corners, minimum height=2cm, minimum width=11cm]
\tikzstyle{context_image} = [rectangle, draw, fill=orange!20, inner sep=0.0mm,
    text width=20em, text centered, rounded corners=2pt, minimum height=1.2cm, minimum width=10cm]
\tikzstyle{context_patch} = [rectangle, draw, fill=orange!20, inner sep=0.0mm,
    text width=0em, text centered, rounded corners=2pt, minimum height=0.5cm, minimum width=0.6cm]
\tikzstyle{canonical_views} = [rectangle, draw, fill=red!20, inner sep=0.0mm,
    text width=10em, text height = 1.8cm, text centered, rounded corners, minimum height=2cm, minimum width=5.1cm]
\tikzstyle{goal_pred} = [rectangle, draw, fill=gray!15, inner sep=0.0mm,
    text width=5em, text height = 1cm, text centered, rounded corners, minimum height=1.2cm, minimum width=2.3cm]
\tikzstyle{query} = [rectangle, draw, fill=gray!5, inner sep=0.0mm,
    text width=4em, text height = 1cm, text centered, rounded corners, minimum height=1.2cm, minimum width=0.8cm]
\tikzstyle{resnet_large} = [rectangle, draw, fill=orange!20, inner sep=0.0mm,
    text width=20em, text centered, rounded corners, minimum height=1cm, minimum width=11cm]
\tikzstyle{resnet_small} = [rectangle, draw, fill=orange!20, inner sep=0.0mm,
    text width=10em, text centered, rounded corners, minimum height=1cm, minimum width=5.1cm]
\tikzstyle{projection_patches} = [rectangle, draw, fill=orange!20, inner sep=0.0mm,
    text width=20em, text centered, rounded corners, minimum height=1cm, minimum width=16.5cm]
\tikzstyle{projection_patch} = [rectangle, draw, fill=orange!20, inner sep=0.0mm,
    text width=0em, text centered, rounded corners=2pt, minimum height=0.5cm, minimum width=0.3cm]
\tikzstyle{projection_patch_description} = [rectangle, draw, fill=red!20, inner sep=0.0mm,
    text width=0.2cm, text centered, rounded corners=2pt, minimum height=0.5cm, minimum width=0.3cm]
\tikzstyle{transformer} = [rectangle, draw, fill=gray!20, inner sep=0.0mm,
    text width=20em, text centered, rounded corners, minimum height=1cm, minimum width=16.5cm]
\tikzstyle{embedding} = [rectangle, draw, fill=purple!20, inner sep=0.0mm,
    text width=0.2cm, text centered, rounded corners=2pt, minimum height=0.809cm, minimum width=0.3cm]
\tikzstyle{readout} = [rectangle, draw, fill=green!10, dashed,
    text width=20em, text depth = 2.6cm, anchor=north, text centered, rounded corners, minimum height=2.6cm, minimum width=16.5cm]
\tikzstyle{dataset} = [rectangle, draw, fill=lime!10, text=black, dashed,
    text width=20em, text depth = 2.6cm, anchor=north, text centered, rounded corners, minimum height=2cm, minimum width=16.5cm]
\tikzstyle{mlp} = [rectangle, draw, fill=white!20, 
    text width=5em, text centered, rounded corners, minimum height=1cm, minimum width=3.4cm]
\tikzstyle{output} = [rectangle, draw, fill=lime!20, 
    text width=5em, text centered, rounded corners, minimum height=1cm, minimum width=2cm]
\tikzstyle{arrow_txt} = [text width=2cm,midway,right=0em,align=left, font={\fontsize{8pt}{12}\selectfont}]

\begin{figure}[!h]
\centering
\resizebox{1\linewidth}{!}{
\begin{tikzpicture}[node distance = 0cm, auto]
    % Place nodes
    \node (cps) [context_patches] {Context Patches};
    \node (cvs) [canonical_views, right=0.4cm of cps] {Canonical Object Views};
    \node (gp) [goal_pred, above=-1.28cm of cvs, xshift=-0.85cm] {Predicate};
    \node (q) [query, right=0.4cm of gp] {Query};
    \node (pps) [projection_patches, above=0.3cm of cps, xshift=2.75cm] {Linear Projection of Flattened Patches};
    
    \node (cp1) [context_patch, above=0cm of pps, xshift=-7.15cm, yshift=-2cm] {};
    \node (cp2) [context_patch, right=0.5cm of cp1] {};
    \node (cp3) [context_patch, right=0.5cm of cp2] {};
    \node (cp4) [context_patch, right=0.5cm of cp3] {};
    \node (cp5) [context_patch, right=0.5cm of cp4] {};
    \node (cp6) [context_patch, right=0.5cm of cp5] {};
    \node (cp7) [context_patch, right=0.5cm of cp6] {};
    \node (cp8) [context_patch, right=0.5cm of cp7] {};
    \node (cp9) [context_patch, right=0.5cm of cp8] {};
    
    \node (qp1) [context_patch, above=0cm of pps, xshift=4.3cm, yshift=-2cm] {};
    \node (qp2) [context_patch, right=0.5cm of qp1] {};
    \node (qp3) [context_patch, right=1.1cm of qp2] {};
    
    \node (pp1) [projection_patch, above=0.2cm of pps, xshift=-7cm] {};
    \node (ppd1) [projection_patch_description, left=0cm of pp1] {1};
    
    \node (pp2) [projection_patch, right=0.8cm of pp1] {};
    \node (ppd2) [projection_patch_description, left=0cm of pp2] {2};
    
    \node (pp3) [projection_patch, right=0.8cm of pp2] {};
    \node (ppd3) [projection_patch_description, left=0cm of pp3] {3};
    
    \node (pp4) [projection_patch, right=0.8cm of pp3] {};
    \node (ppd4) [projection_patch_description, left=0cm of pp4] {4};
    
    \node (pp5) [projection_patch, right=0.8cm of pp4] {};
    \node (ppd5) [projection_patch_description, left=0cm of pp5] {5};
    
    \node (pp6) [projection_patch, right=0.8cm of pp5] {};
    \node (ppd6) [projection_patch_description, left=0cm of pp6] {6};
    
    \node (pp7) [projection_patch, right=0.8cm of pp6] {};
    \node (ppd7) [projection_patch_description, left=0cm of pp7] {7};
    
    \node (pp8) [projection_patch, right=0.8cm of pp7] {};
    \node (ppd8) [projection_patch_description, left=0cm of pp8] {8};
    
    \node (pp9) [projection_patch, right=0.8cm of pp8] {};
    \node (ppd9) [projection_patch_description, left=0cm of pp9] {9};
    
    % query
    \node (q1) [projection_patch, above=0.2cm of pps, xshift=4.45cm] {};
    \node (qm1) [projection_patch_description, left=0cm of q1] {0};
    
    \node (q2) [projection_patch, right=0.8cm of q1] {};
    \node (qm2) [projection_patch_description, left=0cm of q2] {0};
    
    \node (q3) [projection_patch, right=1.4cm of q2] {};
    \node (qm3) [projection_patch_description, left=0cm of q3] {0};
    
    % transformer
    \node (transformer) [transformer, above=1cm of pps] {Transformer};
    
    % embedding
    \node (eb1) [embedding, above=0.2cm of transformer, xshift=4.45cm, fill=red!50] {};
    \node (eb2) [embedding, right=0.8cm of eb1, fill=green!50] {};
    \node (eb3) [embedding, right=1.4cm of eb2, fill=cyan!50] {};
    
    % MPL
    \node (readout) [readout, above=1.2cm of transformer] {PEs};
    \node (mlp1) [mlp, above=2.5cm of transformer, xshift=-5.9cm, fill=red!25] {PE1};
    \node (mlp2) [mlp, right=0.5cm of mlp1, fill=teal!25] {PE2};
    \node (mlp3) [mlp, right=0.5cm of mlp2, fill=blue!25] {PE3};
    \node (mlp4) [mlp, right=0.5cm of mlp3, fill=brown!25] {PE4};
    
    % Output
    \node (output1) [output, above=1.5cm of mlp1, fill=red!50] {Left};
    \node (output2) [output, above=1.5cm of mlp2, fill=teal!50] {Right};
    \node (output3) [output, above=1.5cm of mlp3, fill=blue!50] {...};
    \node (output4) [output, above=1.5cm of mlp4, fill=brown!50] {...};
    
    % Draw edges
    \path [arrow] (cp1.north) -- (cp1|-pps.south);
    \path [arrow] (cp2.north) -- (cp2|-pps.south);
    \path [arrow] (cp3.north) -- (cp3|-pps.south);
    \path [arrow] (cp4.north) -- (cp4|-pps.south);
    \path [arrow] (cp5.north) -- (cp5|-pps.south);
    \path [arrow] (cp6.north) -- (cp6|-pps.south);
    \path [arrow] (cp7.north) -- (cp7|-pps.south);
    \path [arrow] (cp8.north) -- (cp8|-pps.south);
    \path [arrow] (cp9.north) -- (cp9|-pps.south);
    
    \path [arrow] (qp1.north) -- (qp1|-pps.south);
    \path [arrow] (qp2.north) -- (qp2|-pps.south);
    \path [arrow] (qp3.north) -- (qp3|-pps.south);
    
    \path [line] (pps.north-|pp1) -- (pp1.south);
    \path [line] (pps.north-|pp2) -- (pp2.south);
    \path [line] (pps.north-|pp3) -- (pp3.south);
    \path [line] (pps.north-|pp4) -- (pp4.south);
    \path [line] (pps.north-|pp5) -- (pp5.south);
    \path [line] (pps.north-|pp6) -- (pp6.south);
    \path [line] (pps.north-|pp7) -- (pp7.south);
    \path [line] (pps.north-|pp8) -- (pp8.south);
    \path [line] (pps.north-|pp9) -- (pp9.south);
    
    \path [line] (pps.north-|q1) -- (q1.south);
    \path [line] (pps.north-|q2) -- (q2.south);
    \path [line] (pps.north-|q3) -- (q3.south);
    
    \path [arrow] (pp1.north) -- (pp1|-transformer.south);
    \path [arrow] (pp2.north) -- (pp2|-transformer.south);
    \path [arrow] (pp3.north) -- (pp3|-transformer.south);
    \path [arrow] (pp4.north) -- (pp4|-transformer.south);
    \path [arrow] (pp5.north) -- (pp5|-transformer.south);
    \path [arrow] (pp6.north) -- (pp6|-transformer.south);
    \path [arrow] (pp7.north) -- (pp7|-transformer.south);
    \path [arrow] (pp8.north) -- (pp8|-transformer.south);
    \path [arrow] (pp9.north) -- (pp9|-transformer.south);
    
    \path [arrow] (q1.north) -- (q1|-transformer.south);
    \path [arrow] (q2.north) -- (q2|-transformer.south);
    \path [arrow] (q3.north) -- (q3|-transformer.south);
    
    \path [line] (transformer.north-|eb1) -- (eb1.south);
    \path [line] (transformer.north-|eb2) -- (eb2.south);
    \path [line] (transformer.north-|eb3) -- (eb3.south);
    
    \path [arrow, line width=0.4mm, color=red!50] (eb1.north) -- ++(0,0.4) -| ([yshift=0cm,xshift=-1cm]mlp1.south);
    \path [arrow, line width=0.4mm, color=red!50] (eb1.north) -- ++(0,0.4) -| ([yshift=0cm,xshift=-1cm]mlp2.south);
    \path [arrow, line width=0.4mm, color=red!50] (eb1.north) -- ++(0,0.4) -| ([yshift=0cm,xshift=-1cm]mlp3.south);
    \path [arrow, line width=0.4mm, color=red!50] (eb1.north) -- ++(0,0.4) -| ([yshift=0cm,xshift=-1cm]mlp4.south);
    
    \path [arrow, line width=0.4mm, color=teal] (eb2.north) -- ++(0,0.7) -| ([yshift=0cm,xshift=0cm]mlp1.south);
    \path [arrow, line width=0.4mm, color=teal] (eb2.north) -- ++(0,0.7) -| ([yshift=0cm,xshift=0cm]mlp2.south);
    \path [arrow, line width=0.4mm, color=teal] (eb2.north) -- ++(0,0.7) -| ([yshift=0cm,xshift=0cm]mlp3.south);
    \path [arrow, line width=0.4mm, color=teal] (eb2.north) -- ++(0,0.7) -| ([yshift=0cm,xshift=0cm]mlp4.south);
    
    \path [arrow, line width=0.4mm, color=cyan] (eb3.north) -- ++(0,1.0) -| ([yshift=0cm,xshift=1cm]mlp1.south);
    \path [arrow, line width=0.4mm, color=cyan] (eb3.north) -- ++(0,1.0) -| ([yshift=0cm,xshift=1cm]mlp2.south);
    \path [arrow, line width=0.4mm, color=cyan] (eb3.north) -- ++(0,1.0) -| ([yshift=0cm,xshift=1cm]mlp3.south);
    \path [arrow, line width=0.4mm, color=cyan] (eb3.north) -- ++(0,1.0) -| ([yshift=0cm,xshift=1cm]mlp4.south);
    
    \path [arrow, line width=0.2mm] (mlp1.north) -- ([yshift=0cm,xshift=0cm]output1.south);
    \path [arrow, line width=0.2mm] (mlp2.north) -- ([yshift=0cm,xshift=0cm]output2.south);
    \path [arrow, line width=0.2mm] (mlp3.north) -- ([yshift=0cm,xshift=0cm]output3.south);
    \path [arrow, line width=0.2mm] (mlp4.north) -- ([yshift=0cm,xshift=0cm]output4.south);

\end{tikzpicture}
}
\caption{\footnotesize The model structure. The input of the whole model consists of two major parts, one is Context Patches which is the picture of the scene, and the other is Canonical Object Views which is the description picture of the object to be queried. In the middle is the very normal Transformer model. Finally, there are four independent PEs, which correspond to different Predicates.}
\label{fig:arch_detailed}
\end{figure}

\begin{figure}[!h]
\centering
\resizebox{1\linewidth}{!}{
\begin{tikzpicture}[node distance = 0cm, auto]
    % Place nodes
    \node (cps) [context_patches] {Context Image};
    \node (cvs) [canonical_views, right=0.4cm of cps] {Canonical Object Views};
    \node (gp) [goal_pred, above=-1.28cm of cvs, xshift=-0.85cm] {Predicate};
    \node (q) [query, right=0.4cm of gp] {Query};
    \node (resnetl) [resnet_large, above=0.3cm of cps, xshift=0cm] {Resnet};
    \node (resnets) [resnet_small, right=0.4cm of resnetl] {Resnet};

    \node (cp1) [context_image, above=-1.28cm of cps, xshift=0cm, yshift=0cm] {Scene Image};
    
    \node (qp1) [context_patch, above=0cm of pps, xshift=4.3cm, yshift=-2cm] {};
    \node (qp2) [context_patch, right=0.5cm of qp1] {};
    \node (qp3) [context_patch, right=1.1cm of qp2] {};
    
    % Dense layer
    \node (denselayer) [transformer, above=0.3cm of pps] {Dense Layer};
    
    % embedding
    \node (eb1) [embedding, above=0.2cm of denselayer, xshift=4.45cm, fill=red!50] {};
    \node (eb2) [embedding, right=0.8cm of eb1, fill=green!50] {};
    \node (eb3) [embedding, right=1.4cm of eb2, fill=cyan!50] {};
    
    % MPL
    \node (readout) [readout, above=1.2cm of denselayer] {PEs};
    \node (mlp1) [mlp, above=2.5cm of denselayer, xshift=-5.9cm, fill=red!25] {PE1};
    \node (mlp2) [mlp, right=0.5cm of mlp1, fill=teal!25] {PE2};
    \node (mlp3) [mlp, right=0.5cm of mlp2, fill=blue!25] {PE3};
    \node (mlp4) [mlp, right=0.5cm of mlp3, fill=brown!25] {PE4};
    
    % Output
    \node (output1) [output, above=1.5cm of mlp1, fill=red!50] {Left};
    \node (output2) [output, above=1.5cm of mlp2, fill=teal!50] {Right};
    \node (output3) [output, above=1.5cm of mlp3, fill=blue!50] {...};
    \node (output4) [output, above=1.5cm of mlp4, fill=brown!50] {...};
    
    % Draw edges
    \path [arrow] (cp1.north) -- (cp1|-resnetl.south);
    
    \path [arrow] (qp1.north) -- (qp1|-resnetl.south);
    \path [arrow] (qp2.north) -- (qp2|-resnetl.south);
    \path [arrow] (qp3.north) -- (qp3|-resnetl.south);
    
    \path [arrow] ([yshift=0cm,xshift=-2.75cm]pps.north) -- ([yshift=0cm,xshift=-2.75cm]denselayer.south);
    
    \path [arrow] ([yshift=0cm,xshift=-1.25cm]resnets.north) -- ([xshift=-1.25cm]resnets.north|-denselayer.south);
    \path [arrow] ([yshift=0cm,xshift=-0.15cm]resnets.north) -- ([xshift=-0.15cm]resnets.north|-denselayer.south);
    \path [arrow] ([yshift=0cm,xshift=1.55cm]resnets.north) -- ([xshift=1.55cm]resnets.north|-denselayer.south);
    
    \path [line] (denselayer.north-|eb1) -- (eb1.south);
    \path [line] (denselayer.north-|eb2) -- (eb2.south);
    \path [line] (denselayer.north-|eb3) -- (eb3.south);
    
    \path [arrow, line width=0.4mm, color=red!50] (eb1.north) -- ++(0,0.4) -| ([yshift=0cm,xshift=-1cm]mlp1.south);
    \path [arrow, line width=0.4mm, color=red!50] (eb1.north) -- ++(0,0.4) -| ([yshift=0cm,xshift=-1cm]mlp2.south);
    \path [arrow, line width=0.4mm, color=red!50] (eb1.north) -- ++(0,0.4) -| ([yshift=0cm,xshift=-1cm]mlp3.south);
    \path [arrow, line width=0.4mm, color=red!50] (eb1.north) -- ++(0,0.4) -| ([yshift=0cm,xshift=-1cm]mlp4.south);
    
    \path [arrow, line width=0.4mm, color=teal] (eb2.north) -- ++(0,0.7) -| ([yshift=0cm,xshift=0cm]mlp1.south);
    \path [arrow, line width=0.4mm, color=teal] (eb2.north) -- ++(0,0.7) -| ([yshift=0cm,xshift=0cm]mlp2.south);
    \path [arrow, line width=0.4mm, color=teal] (eb2.north) -- ++(0,0.7) -| ([yshift=0cm,xshift=0cm]mlp3.south);
    \path [arrow, line width=0.4mm, color=teal] (eb2.north) -- ++(0,0.7) -| ([yshift=0cm,xshift=0cm]mlp4.south);
    
    \path [arrow, line width=0.4mm, color=cyan] (eb3.north) -- ++(0,1.0) -| ([yshift=0cm,xshift=1cm]mlp1.south);
    \path [arrow, line width=0.4mm, color=cyan] (eb3.north) -- ++(0,1.0) -| ([yshift=0cm,xshift=1cm]mlp2.south);
    \path [arrow, line width=0.4mm, color=cyan] (eb3.north) -- ++(0,1.0) -| ([yshift=0cm,xshift=1cm]mlp3.south);
    \path [arrow, line width=0.4mm, color=cyan] (eb3.north) -- ++(0,1.0) -| ([yshift=0cm,xshift=1cm]mlp4.south);
    
    \path [arrow, line width=0.2mm] (mlp1.north) -- ([yshift=0cm,xshift=0cm]output1.south);
    \path [arrow, line width=0.2mm] (mlp2.north) -- ([yshift=0cm,xshift=0cm]output2.south);
    \path [arrow, line width=0.2mm] (mlp3.north) -- ([yshift=0cm,xshift=0cm]output3.south);
    \path [arrow, line width=0.2mm] (mlp4.north) -- ([yshift=0cm,xshift=0cm]output4.south);

\end{tikzpicture}
}
\caption{\footnotesize The model structure which base on the ResNet. The model input is also divided into two parts, Context Image and Canonical Object Views. Context Image is not split into patches. In addition, the input images will be processed by two ResNet of different scales.}
\label{fig:arch_detailed_resnet}
\end{figure}

\begin{figure}[!h]
\centering
\resizebox{1\linewidth}{!}{
\begin{tikzpicture}[node distance = 0cm, auto]
    % Place nodes
    \node (cps) [context_patches] {Context Patches};
    \node (cvs) [canonical_views, right=0.4cm of cps] {Canonical Object Views};
    \node (gp) [goal_pred, above=-1.28cm of cvs, xshift=-0.85cm] {Predicate};
    \node (q) [query, right=0.4cm of gp] {Query};
    \node (pps) [projection_patches, above=0.3cm of cps, xshift=2.75cm] {3-dimensional Residual Neural Network};
    
    \node (cp1) [context_patch, above=0cm of pps, xshift=-7.15cm, yshift=-2cm] {};
    \node (cp2) [context_patch, right=0.5cm of cp1] {};
    \node (cp3) [context_patch, right=0.5cm of cp2] {};
    \node (cp4) [context_patch, right=0.5cm of cp3] {};
    \node (cp5) [context_patch, right=0.5cm of cp4] {};
    \node (cp6) [context_patch, right=0.5cm of cp5] {};
    \node (cp7) [context_patch, right=0.5cm of cp6] {};
    \node (cp8) [context_patch, right=0.5cm of cp7] {};
    \node (cp9) [context_patch, right=0.5cm of cp8] {};
    
    \node (qp1) [context_patch, above=0cm of pps, xshift=4.3cm, yshift=-2cm] {};
    \node (qp2) [context_patch, right=0.5cm of qp1] {};
    \node (qp3) [context_patch, right=1.1cm of qp2] {};
    
    % Dense Layer
    \node (denselayer) [transformer, above=0.3cm of pps] {Dense Layer};
    
    % embedding
    \node (eb1) [embedding, above=0.2cm of denselayer, xshift=4.45cm, fill=red!50] {};
    \node (eb2) [embedding, right=0.8cm of eb1, fill=green!50] {};
    \node (eb3) [embedding, right=1.4cm of eb2, fill=cyan!50] {};
    
    % MPL
    \node (readout) [readout, above=1.2cm of denselayer] {PEs};
    \node (mlp1) [mlp, above=2.5cm of denselayer, xshift=-5.9cm, fill=red!25] {PE1};
    \node (mlp2) [mlp, right=0.5cm of mlp1, fill=teal!25] {PE2};
    \node (mlp3) [mlp, right=0.5cm of mlp2, fill=blue!25] {PE3};
    \node (mlp4) [mlp, right=0.5cm of mlp3, fill=brown!25] {PE4};
    
    % Output
    \node (output1) [output, above=1.5cm of mlp1, fill=red!50] {Left};
    \node (output2) [output, above=1.5cm of mlp2, fill=teal!50] {Right};
    \node (output3) [output, above=1.5cm of mlp3, fill=blue!50] {...};
    \node (output4) [output, above=1.5cm of mlp4, fill=brown!50] {...};
    
    % Draw edges
    \path [arrow] (cp1.north) -- (cp1|-pps.south);
    \path [arrow] (cp2.north) -- (cp2|-pps.south);
    \path [arrow] (cp3.north) -- (cp3|-pps.south);
    \path [arrow] (cp4.north) -- (cp4|-pps.south);
    \path [arrow] (cp5.north) -- (cp5|-pps.south);
    \path [arrow] (cp6.north) -- (cp6|-pps.south);
    \path [arrow] (cp7.north) -- (cp7|-pps.south);
    \path [arrow] (cp8.north) -- (cp8|-pps.south);
    \path [arrow] (cp9.north) -- (cp9|-pps.south);
    
    \path [arrow] (qp1.north) -- (qp1|-pps.south);
    \path [arrow] (qp2.north) -- (qp2|-pps.south);
    \path [arrow] (qp3.north) -- (qp3|-pps.south);
    
    \path [arrow] (pps.north) -- (pps|-denselayer.south);
    
    \path [line] (denselayer.north-|eb1) -- (eb1.south);
    \path [line] (denselayer.north-|eb2) -- (eb2.south);
    \path [line] (denselayer.north-|eb3) -- (eb3.south);
    
    \path [arrow, line width=0.4mm, color=red!50] (eb1.north) -- ++(0,0.4) -| ([yshift=0cm,xshift=-1cm]mlp1.south);
    \path [arrow, line width=0.4mm, color=red!50] (eb1.north) -- ++(0,0.4) -| ([yshift=0cm,xshift=-1cm]mlp2.south);
    \path [arrow, line width=0.4mm, color=red!50] (eb1.north) -- ++(0,0.4) -| ([yshift=0cm,xshift=-1cm]mlp3.south);
    \path [arrow, line width=0.4mm, color=red!50] (eb1.north) -- ++(0,0.4) -| ([yshift=0cm,xshift=-1cm]mlp4.south);
    
    \path [arrow, line width=0.4mm, color=teal] (eb2.north) -- ++(0,0.7) -| ([yshift=0cm,xshift=0cm]mlp1.south);
    \path [arrow, line width=0.4mm, color=teal] (eb2.north) -- ++(0,0.7) -| ([yshift=0cm,xshift=0cm]mlp2.south);
    \path [arrow, line width=0.4mm, color=teal] (eb2.north) -- ++(0,0.7) -| ([yshift=0cm,xshift=0cm]mlp3.south);
    \path [arrow, line width=0.4mm, color=teal] (eb2.north) -- ++(0,0.7) -| ([yshift=0cm,xshift=0cm]mlp4.south);
    
    \path [arrow, line width=0.4mm, color=cyan] (eb3.north) -- ++(0,1.0) -| ([yshift=0cm,xshift=1cm]mlp1.south);
    \path [arrow, line width=0.4mm, color=cyan] (eb3.north) -- ++(0,1.0) -| ([yshift=0cm,xshift=1cm]mlp2.south);
    \path [arrow, line width=0.4mm, color=cyan] (eb3.north) -- ++(0,1.0) -| ([yshift=0cm,xshift=1cm]mlp3.south);
    \path [arrow, line width=0.4mm, color=cyan] (eb3.north) -- ++(0,1.0) -| ([yshift=0cm,xshift=1cm]mlp4.south);
    
    \path [arrow, line width=0.2mm] (mlp1.north) -- ([yshift=0cm,xshift=0cm]output1.south);
    \path [arrow, line width=0.2mm] (mlp2.north) -- ([yshift=0cm,xshift=0cm]output2.south);
    \path [arrow, line width=0.2mm] (mlp3.north) -- ([yshift=0cm,xshift=0cm]output3.south);
    \path [arrow, line width=0.2mm] (mlp4.north) -- ([yshift=0cm,xshift=0cm]output4.south);

\end{tikzpicture}
}
\caption{\footnotesize The model structure which base on the three-dimensional ResNet. The inputs to this model are consistent with the Transformer-based model. It is finally converted into the corresponding output through a three-dimensional network of residuals and a fully connected layer.}
\label{fig:arch_detailed_resnet_3d}
\end{figure}

\begin{figure}[!h]
\centering
\resizebox{1\linewidth}{!}{
\begin{tikzpicture}[node distance = 0cm, auto]
    % transformer
    \node (transformer) [transformer, above=1cm of pps] {Transformer};
    
    % MPL
    \node (readout) [readout, above=1.2cm of transformer] {PEs};
    \node (mlp1) [mlp, above=2.5cm of transformer, xshift=-5.9cm, fill=red!25] {PE1};
    \node (mlp2) [mlp, right=0.5cm of mlp1, fill=teal!25] {PE2};
    \node (mlp3) [mlp, right=0.5cm of mlp2, fill=blue!25] {PE3};
    \node (mlp4) [mlp, right=0.5cm of mlp3, fill=brown!25] {PE4};
    
    %Dataset
    \node (dataset, minimum height=2.6cm) [dataset, above=1.2cm of readout] {Datasets};
    \node (data1) [mlp, above=2.5cm of readout, xshift=-5.9cm, fill=red!50] {dataset1};
    \node (data2) [mlp, right=0.5cm of data1, fill=teal!50] {dataset2};
    \node (data3) [mlp, right=0.5cm of data2, fill=blue!50] {dataset3};
    \node (data4) [mlp, right=0.5cm of data3, fill=brown!50] {dataset4};
    
    % Draw edges

    \path [arrow, line width=1.5mm, color=red] (mlp1.south) -- ++(0,-1.6) -| ([yshift=0cm,xshift=0cm]transformer.north);
    \path [arrow, line width=1.5mm, color=teal] (mlp2.south) -- ++(0,-0.7) -| ([yshift=0cm,xshift=0cm]transformer.north);
    \path [arrow, line width=1.5mm, color=blue] (mlp3.south) -- ++(0,-0.9) -| ([yshift=0cm,xshift=0cm]transformer.north);
    \path [arrow, line width=1.5mm, color=brown] (mlp4.south) -- ++(0,-1.1) -| ([yshift=0cm,xshift=0cm]transformer.north);

    \path [arrow, line width=1.5mm, color=red] (data1.south) -- node [text width=2.5cm,midway,right=0em,align=left ] {1.} ([yshift=0cm,xshift=0cm]mlp1.north);
    \path [arrow, line width=1.5mm, color=teal] (data2.south) -- node [text width=2.5cm,midway,right=0em,align=left ] {2.} ([yshift=0cm,xshift=0cm]mlp2.north);
    \path [arrow, line width=1.5mm, color=blue] (data3.south) -- node [text width=2.5cm,midway,right=0em,align=left ] {3.} ([yshift=0cm,xshift=0cm]mlp3.north);
    \path [arrow, line width=1.5mm, color=brown] (data4.south) -- node [text width=2.5cm,midway,right=0em,align=left ] {4.} ([yshift=0cm,xshift=0cm]mlp4.north);
\end{tikzpicture}
}
\caption{Training Procedure with training set as a whole. This training is done by taking one data set as a whole. The next dataset is not used until one dataset has been used.}
\label{fig:training_method_1}
\end{figure}

\begin{figure}[!h]
\centering
\resizebox{1\linewidth}{!}{
\begin{tikzpicture}[node distance = 0cm, auto]
    % transformer
    \node (transformer) [transformer, above=1cm of pps] {Transformer};
    
    % MPL
    \node (readout) [readout, above=1.2cm of transformer] {PEs};
    \node (mlp1) [mlp, above=2.5cm of transformer, xshift=-5.9cm, fill=red!25] {PE1};
    \node (mlp2) [mlp, right=0.5cm of mlp1, fill=teal!25] {PE2};
    \node (mlp3) [mlp, right=0.5cm of mlp2, fill=blue!25] {PE3};
    \node (mlp4) [mlp, right=0.5cm of mlp3, fill=brown!25] {PE4};
    
    %Dataset
    \node (dataset, minimum height=2.6cm) [dataset, above=1.2cm of readout] {Datasets};
    \node (data1) [mlp, above=2.5cm of readout, xshift=-5.9cm, fill=red!50] {dataset1};
    \node (data2) [mlp, right=0.5cm of data1, fill=teal!50] {dataset2};
    \node (data3) [mlp, right=0.5cm of data2, fill=blue!50] {dataset3};
    \node (data4) [mlp, right=0.5cm of data3, fill=brown!50] {dataset4};
    
    % Draw edges

    \path [arrow, line width=0.1mm, color=red] ([yshift=0cm,xshift=-1cm]mlp1.south) -- ++(0,-1.6) -| ([yshift=0cm,xshift=-1cm]transformer.north);
    \path [arrow, line width=0.1mm, color=teal] ([yshift=0cm,xshift=-1cm]mlp2.south) -- ++(0,-0.7) -| ([yshift=0cm,xshift=-1cm]transformer.north);
    \path [arrow, line width=0.1mm, color=blue] ([yshift=0cm,xshift=-1cm]mlp3.south) -- ++(0,-0.9) -| ([yshift=0cm,xshift=-1cm]transformer.north);
    \path [arrow, line width=0.1mm, color=brown] ([yshift=0cm,xshift=-1cm]mlp4.south) -- ++(0,-1.1) -| ([yshift=0cm,xshift=-1cm]transformer.north);
    
    \path [arrow, line width=0.1mm, color=red] ([yshift=0cm,xshift=0cm]mlp1.south) -- ++(0,-1.6) -| ([yshift=0cm,xshift=0cm]transformer.north);
    \path [arrow, line width=0.1mm, color=teal] ([yshift=0cm,xshift=0cm]mlp2.south) -- ++(0,-0.7) -| ([yshift=0cm,xshift=0cm]transformer.north);
    \path [arrow, line width=0.1mm, color=blue] ([yshift=0cm,xshift=0cm]mlp3.south) -- ++(0,-0.9) -| ([yshift=0cm,xshift=0cm]transformer.north);
    \path [arrow, line width=0.1mm, color=brown] ([yshift=0cm,xshift=0cm]mlp4.south) -- ++(0,-1.1) -| ([yshift=0cm,xshift=0cm]transformer.north);
    
    \path [arrow, line width=0.1mm, color=red] ([yshift=0cm,xshift=1cm]mlp1.south) -- ++(0,-1.6) -| ([yshift=0cm,xshift=1cm]transformer.north);
    \path [arrow, line width=0.1mm, color=teal] ([yshift=0cm,xshift=1cm]mlp2.south) -- ++(0,-0.7) -| ([yshift=0cm,xshift=1cm]transformer.north);
    \path [arrow, line width=0.1mm, color=blue] ([yshift=0cm,xshift=1cm]mlp3.south) -- ++(0,-0.9) -| ([yshift=0cm,xshift=1cm]transformer.north);
    \path [arrow, line width=0.1mm, color=brown] ([yshift=0cm,xshift=1cm]mlp4.south) -- ++(0,-1.1) -| ([yshift=0cm,xshift=1cm]transformer.north);

    \path [arrow, line width=0.1mm, color=red] ([yshift=0cm,xshift=-1cm]data1.south) -- ++(0,-1.6) -| node [arrow_txt] {1.} ([yshift=0cm,xshift=-1cm]mlp1.north);
    \path [arrow, line width=0.1mm, color=teal] ([yshift=0cm,xshift=-1cm]data2.south) -- ++(0,-1.6) -| node [arrow_txt] {2.} ([yshift=0cm,xshift=-1cm]mlp2.north);
    \path [arrow, line width=0.1mm, color=blue] ([yshift=0cm,xshift=-1cm]data3.south) -- ++(0,-1.6) -| node [arrow_txt] {3.} ([yshift=0cm,xshift=-1cm]mlp3.north);
    \path [arrow, line width=0.1mm, color=brown] ([yshift=0cm,xshift=-1cm]data4.south) -- ++(0,-1.6) -| node [arrow_txt] {4.} ([yshift=0cm,xshift=-1cm]mlp4.north);
    
    \path [arrow, line width=0.1mm, color=red] ([yshift=0cm,xshift=0cm]data1.south) -- ++(0,-1.6) -| node [arrow_txt] {5.} ([yshift=0cm,xshift=0cm]mlp1.north);
    \path [arrow, line width=0.1mm, color=teal] ([yshift=0cm,xshift=0cm]data2.south) -- ++(0,-1.6) -| node [arrow_txt] {6.} ([yshift=0cm,xshift=0cm]mlp2.north);
    \path [arrow, line width=0.1mm, color=blue] ([yshift=0cm,xshift=0cm]data3.south) -- ++(0,-1.6) -| node [arrow_txt] {7.} ([yshift=0cm,xshift=0cm]mlp3.north);
    \path [arrow, line width=0.1mm, color=brown] ([yshift=0cm,xshift=0cm]data4.south) -- ++(0,-1.6) -| node [arrow_txt] {8.} ([yshift=0cm,xshift=0cm]mlp4.north);
    
    \path [arrow, line width=0.1mm, color=red] ([yshift=0cm,xshift=1cm]data1.south) -- ++(0,-1.6) -| node [arrow_txt] {9...} ([yshift=0cm,xshift=1cm]mlp1.north);
    \path [arrow, line width=0.1mm, color=teal] ([yshift=0cm,xshift=1cm]data2.south) -- ++(0,-1.6) -| node [arrow_txt] {10...} ([yshift=0cm,xshift=1cm]mlp2.north);
    \path [arrow, line width=0.1mm, color=blue] ([yshift=0cm,xshift=1cm]data3.south) -- ++(0,-1.6) -| node [arrow_txt] {11...} ([yshift=0cm,xshift=1cm]mlp3.north);
    \path [arrow, line width=0.1mm, color=brown] ([yshift=0cm,xshift=1cm]data4.south) -- ++(0,-1.6) -| node [arrow_txt] {12...} ([yshift=0cm,xshift=1cm]mlp4.north);
    
\end{tikzpicture}
}
\caption{The batch polling training Procedure}
\label{fig:training_method_2}
\end{figure}

\begin{table}[!h]
\centering
\begin{tabular}{||c c c||} 
\hline
& relevant (pct.) & irrelevant (pct.) \\ [0.5ex] 
% \hline\hline
% Train\_left\_7obj       & 349271 (17.8\%) & 1610729 (82.2\%) \\ 
% Train\_right\_7obj      & 349155 (17.8\%) & 1610845 (82.2\%) \\
% Train\_in\_front\_7obj  & 349951 (17.9\%) & 1610049 (82.1\%) \\
% Train\_behind\_7obj     & 349423 (17.8\%) & 1610577 (82.2\%) \\
% Test\_left\_7obj        & 3506 (17.9\%) & 16094 (82.1\%) \\
% Test\_right\_7obj       & 3484 (17.8\%) & 16116 (82.2\%) \\
% Test\_in\_front\_7obj   & 3513 (17.9\%) & 16087 (82.1\%) \\
% Test\_behind\_7obj      & 3464 (17.7\%) & 16136 (82.3\%) \\
\hline\hline
Train\_left\_10obj       & 1235677 (13.7\%) & 7764323 (86.3\%) \\ 
Train\_right\_10obj      & 1239533 (13.8\%) & 7760467 (86.2\%) \\
Train\_in\_front\_10obj  & 1239388 (13.8\%) & 7760612 (86.2\%) \\
Train\_behind\_10obj     & 1248629 (13.9\%) & 7751371 (86.1\%) \\
Test\_left\_10obj        & 12448 (13.8\%) & 77552 (86.2\%) \\
Test\_right\_10obj       & 12557 (14.0\%) & 77443 (86.0\%) \\
Test\_in\_front\_10obj   & 12401 (13.8\%) & 77599 (86.2\%) \\
Test\_behind\_10obj      & 12495 (13.9\%) & 77505 (86.1\%) \\
\hline\hline
Train\_on   & 3650855 (30.4\%) & 8349145 (69.6\%) \\ 
Test\_on    & 34689 (28.9\%) & 85311 (71.1\%) \\
\hline
\end{tabular}
\caption{Distribution of labels in each dataset}
\label{tbl:datasets_overview}
\end{table}
